# Supplementary material for: Sequential Search with Off-Policy Reinforcement Learning
Source: arXiv:2202.00245 source file (2022-02-01)
Supplement: Supplementary file 1 [file 7-appendix.tex]

\section{Appendix}
